# Supplementary material for: Review of deep learning models for crypto price prediction: implementation and evaluation
Source: arXiv:2405.11431 source file (2024-06-02)
Supplement: Supplementary file 1 [file appendix1.tex]

Rate each team member's overall contribution to the Group Project

Name of group member - Percentage of contribution:

Jingyang Wu - 32.5\%
Xinyi Zhang - 32.5\%
Fangyixuan Huang - 17.5\%
Haochen Zhou - 17.5\%
